# Supplementary material for: A Power Analysis of the Conditional Randomization Test and Knockoffs
Source: arXiv:2010.02304 source file (2020-10-05)
Supplement: Supplementary file 1 [file knockoffs.tex]

\section{Quality of the knockoffs}
\label{sec:knock-qual}
It has been observed and noted that the quality of the knockoffs plays an important role its performance \citep{candes2018panning,SB-EC-LJ-WW:2020}. In this section, we discuss how the quality of the knockoffs affects power. We focus on the correlation between the covariates and their knockoff counterparts, as suggested in \citet{candes2018panning}. It should be clear from the previous section that in order to achieve high power, the non-null $p$-values should have very different distributions than the null $p$-values. To better understand the mechanism, consider %a toy setting where we have $p$ independent statistic $T_j\sim\mathcal N(\theta_j,1)$, with $\gamma$ fraction of $\theta_j$'s being $0$ and $(1-\gamma)$ being $h$. Suppose we have knockoff statistics $T_{j+p}$ from $\mathcal N(0,1)$, jointly normal with $T_j$ with correlation $\rho$ and independent of the other $T_j$'s. This can be thought of as
a linear regression case where each non-null $\beta_j=h/\sqrt{n}$, the error variance is $1$, $n\gg p$, and independently for each $j$ we have
\begin{equation*}
\left(
  \begin{array}{c}
X_j\\
\tilde X_j\\
  \end{array}
\right)\sim\mathcal N\left(\left(
  \begin{array}{c}
0\\
0\\
  \end{array}
\right),\left[
  \begin{array}{cc}
1 & -\rho\\
-\rho & 1\\
  \end{array}
\right]\right).
\end{equation*}
Suppose we let the variable importance statistic be $W_j=\sqrt n(|\hat\beta_j|-|\hat\beta_{j+p}|)$. If we let $F_{\mu,\rho}$ be the distribution of $|X|-|Y|$, where
\begin{equation*}
\left(
  \begin{array}{c}
X\\
Y\\
  \end{array}
\right)\sim\mathcal N\left(\left(
  \begin{array}{c}
\mu\\
0\\
  \end{array}
\right),\left[
  \begin{array}{cc}
1 & \rho\\
\rho & 1\\
  \end{array}
\right]\right),
\end{equation*}
then it can be seen that the null $W_j=\sqrt n(\hat\beta_j-\hat\beta_{j+p})$ has distribution $(1-\rho^2)^{-1/2}F_{0,\rho}$, and the non-null $W_j$ has distribution $(1-\rho^2)^{-1/2}F_{h\sqrt{1-\rho^2},\rho}$. = Intuitively, we can expect high power if $F_{h\sqrt{1-\rho^2},\rho}$ is quite different from $(1-\rho^2)^{-1/2}F_{0,\rho}$, which should occur when $|\rho|$ is low. In Figure~\ref{fig:compare-rhos}, we compare the two distributions for different $\rho$. The two distributions become more entangled as $\rho$ grows, while the change is flat when $\rho$ is small.

Note that
\begin{equation*}
\begin{aligned}
F_{\mu,\rho}(x)&=1-\p(\{X-Y\ge x,X+Y\ge x\}\cup\{X+Y\le-x,X-Y\le-x\})\\
&=1-\p(X-Y\ge x,X+Y\ge x)-\p(X+Y\le-x,X-Y\le-x)\\
&\quad+\p(X-Y\ge x,X+Y\ge x,X+Y\le-x,X-Y\le-x)\\
&=1-\Phi(\frac{\mu-x}{\sqrt{2(1+\rho)}})\Phi(\frac{\mu-x}{\sqrt{2(1-\rho)}})-\Phi(\frac{-\mu-x}{\sqrt{2(1+\rho)}})\Phi(\frac{-\mu-x}{\sqrt{2(1-\rho)}})\\
&\quad+\mathbb I(x<0)\left[\Phi(\frac{-x-\mu}{\sqrt{2(1+\rho)}})-\Phi(\frac{x-\mu}{\sqrt{2(1+\rho)}})\right]\left[\Phi(\frac{-x-\mu}{\sqrt{2(1-\rho)}})-\Phi(\frac{x-\mu}{\sqrt{2(1-\rho)}})\right].
\end{aligned}
\end{equation*}

% Let
% \begin{equation*}
% \begin{aligned}
% \tau_\text{KF}&=\min\{t>0:\frac{1+\#\{j:W_j\le-t\}}{\#\{j:W_j\ge t\}}\ge q\}\\
% &\approx\min\{t>0:\frac{\gamma F_{0,\rho}(-t)+(1-\gamma)F_{h\sqrt{n(1-\rho^2)},\rho}(-t)}{\gamma F_{0,\rho}(-t)+(1-\gamma)(1-F_{h\sqrt{n(1-\rho^2)},\rho}(t))}\le q\},
% \end{aligned}
% \end{equation*}
% and the power is $1-F_{h\sqrt{n(1-\rho^2)},\rho}(\tau_\text{KF})$.

\begin{figure}[h]
     \centering
     \begin{subfigure}[b]{0.3\textwidth}
         \centering
         \includegraphics[width=\textwidth]{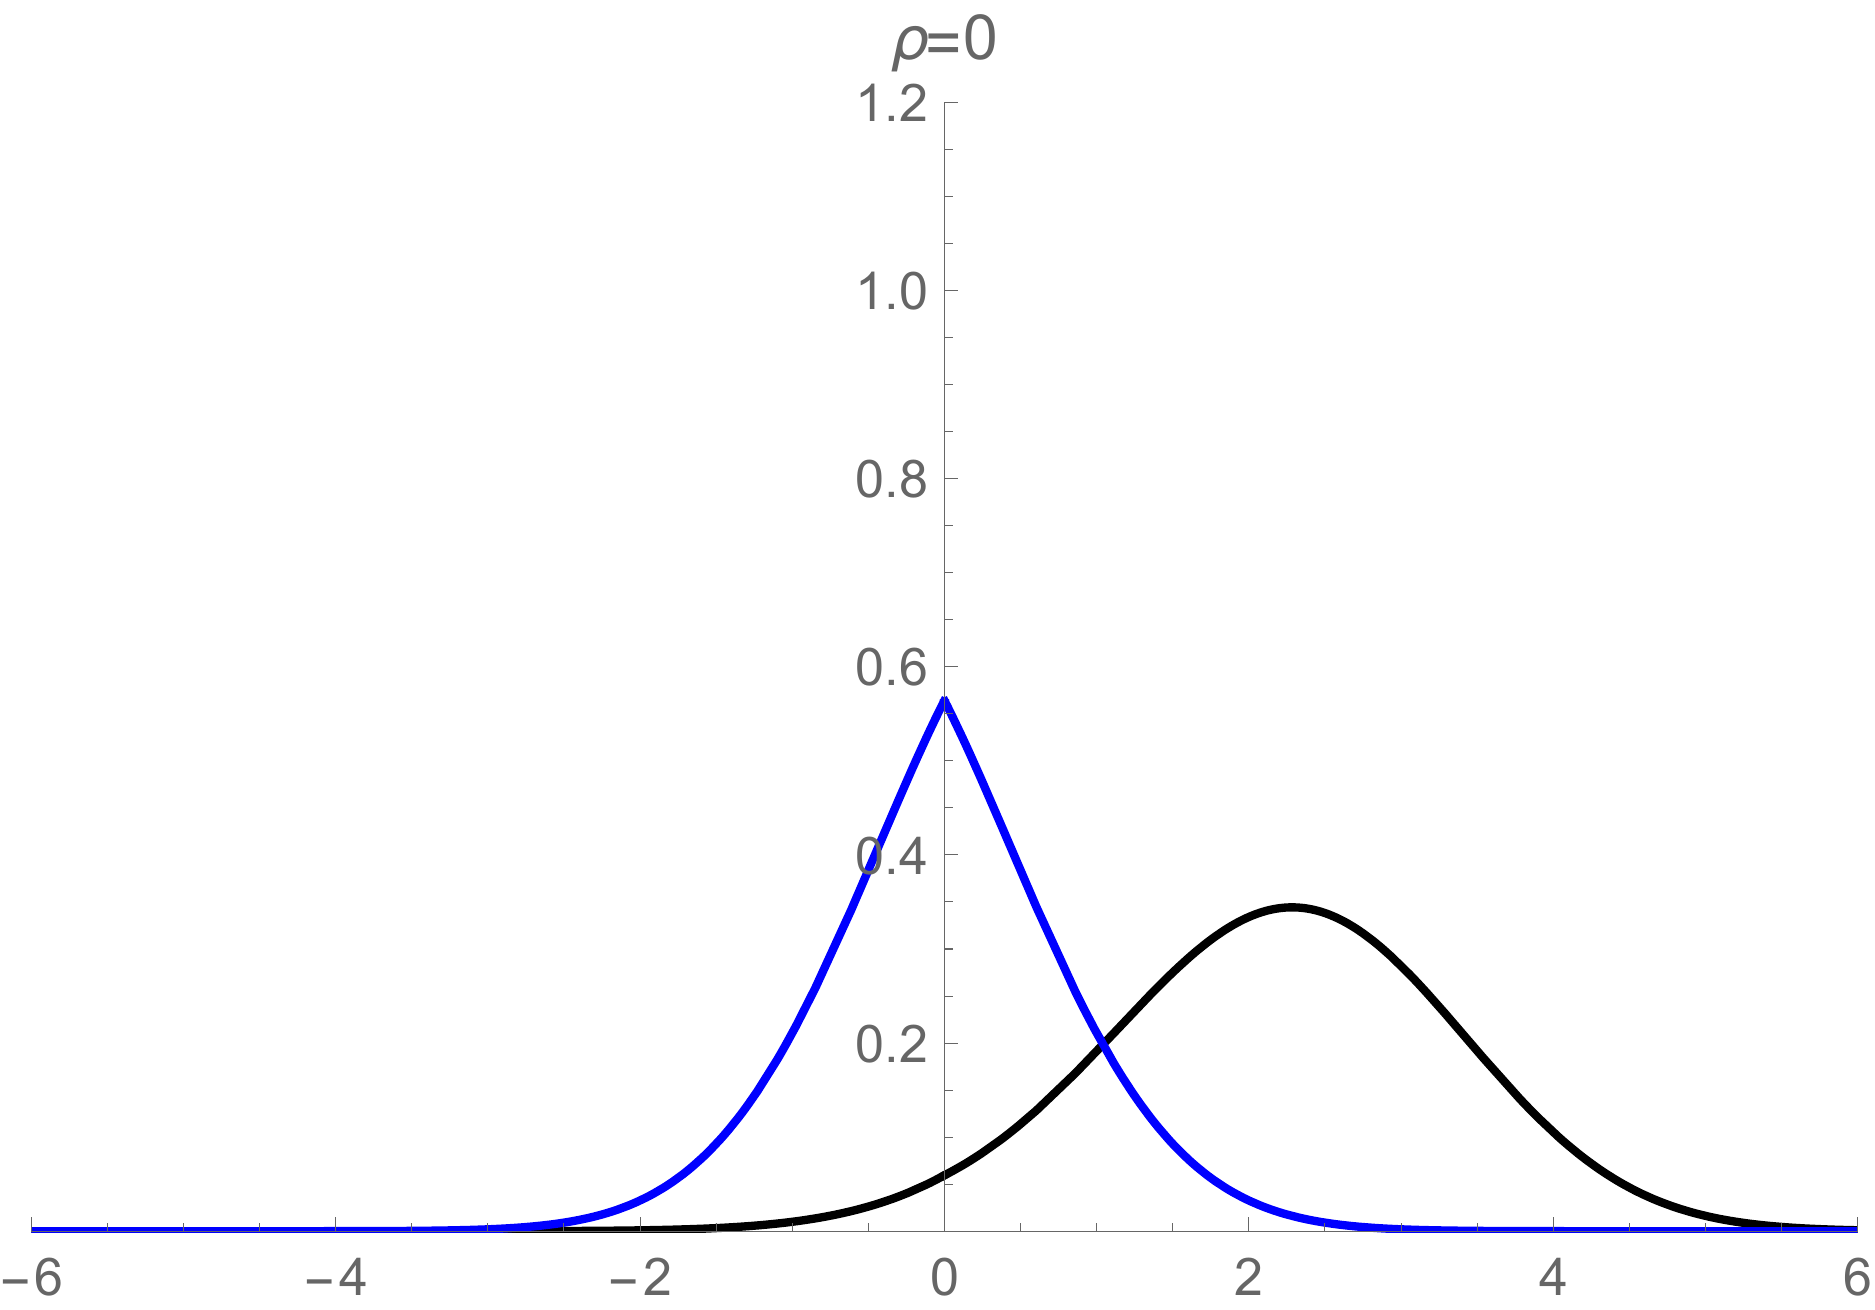}
         \caption{$\rho=0$}
     \end{subfigure}
     \hfill
     \begin{subfigure}[b]{0.3\textwidth}
         \centering
         \includegraphics[width=\textwidth]{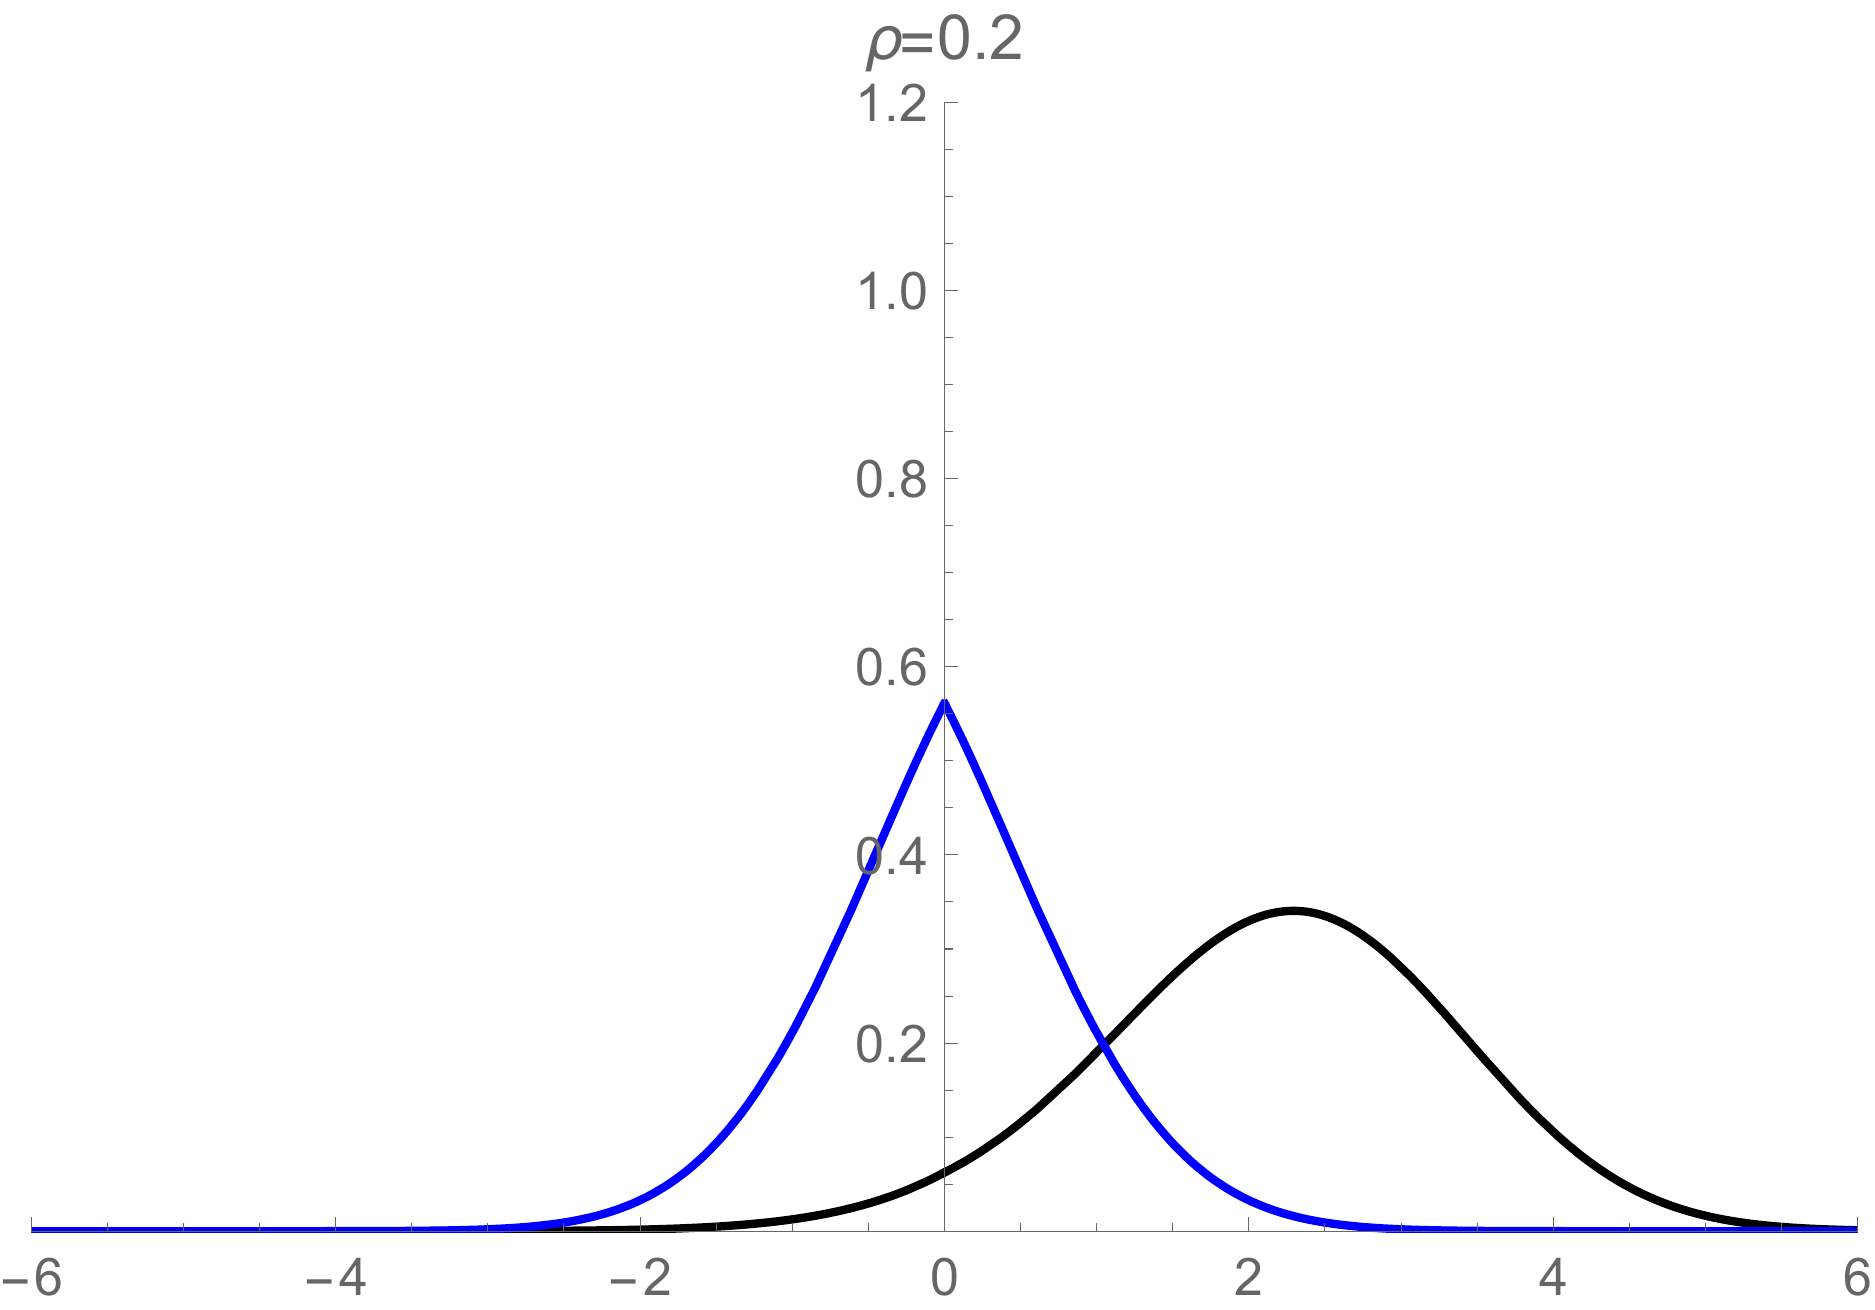}
         \caption{$\rho=0.2$}
     \end{subfigure}
     \hfill
     \begin{subfigure}[b]{0.3\textwidth}
         \centering
         \includegraphics[width=\textwidth]{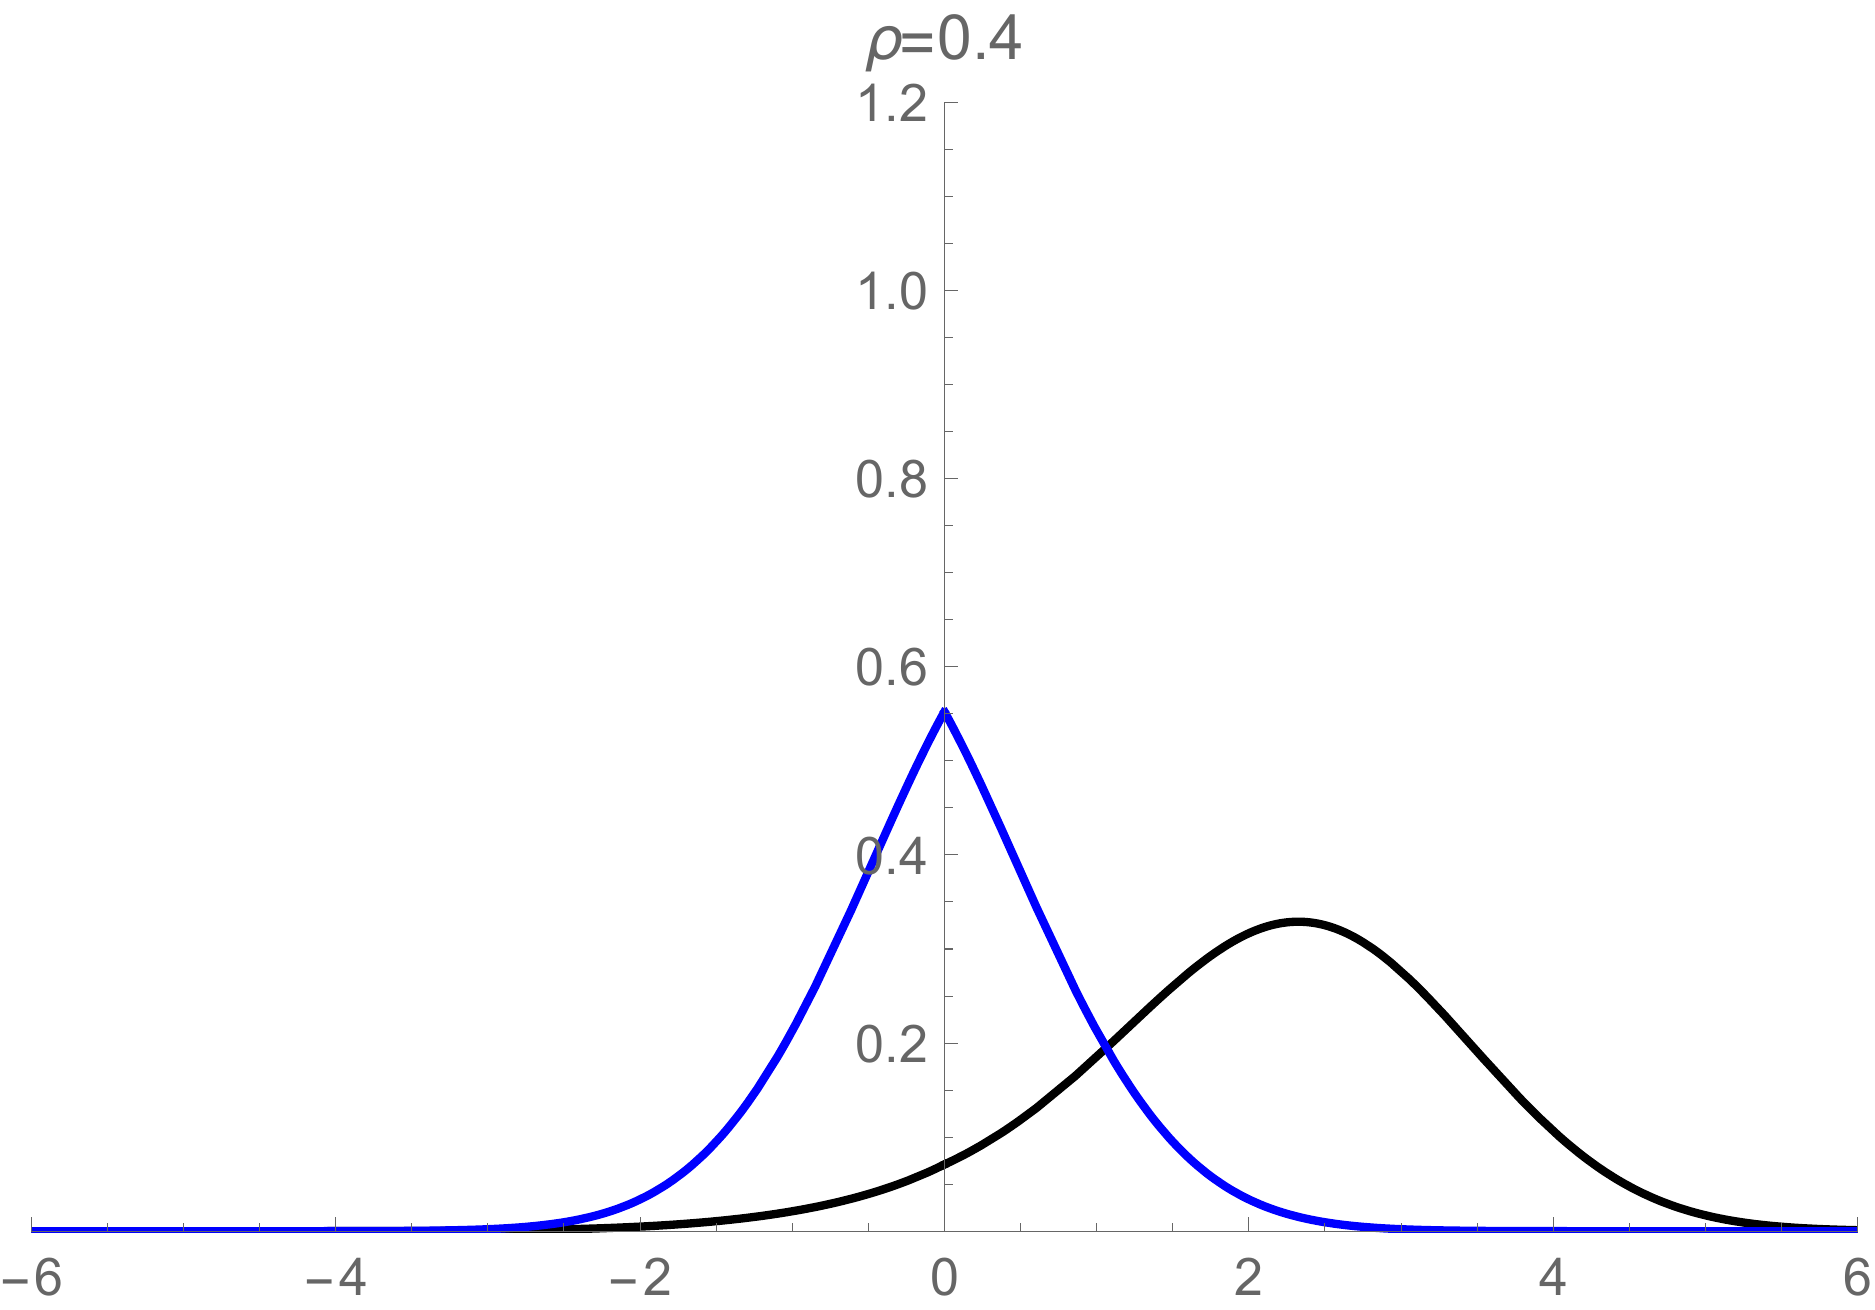}
         \caption{$\rho=0.4$}
     \end{subfigure}
     \begin{subfigure}[b]{0.3\textwidth}
         \centering
         \includegraphics[width=\textwidth]{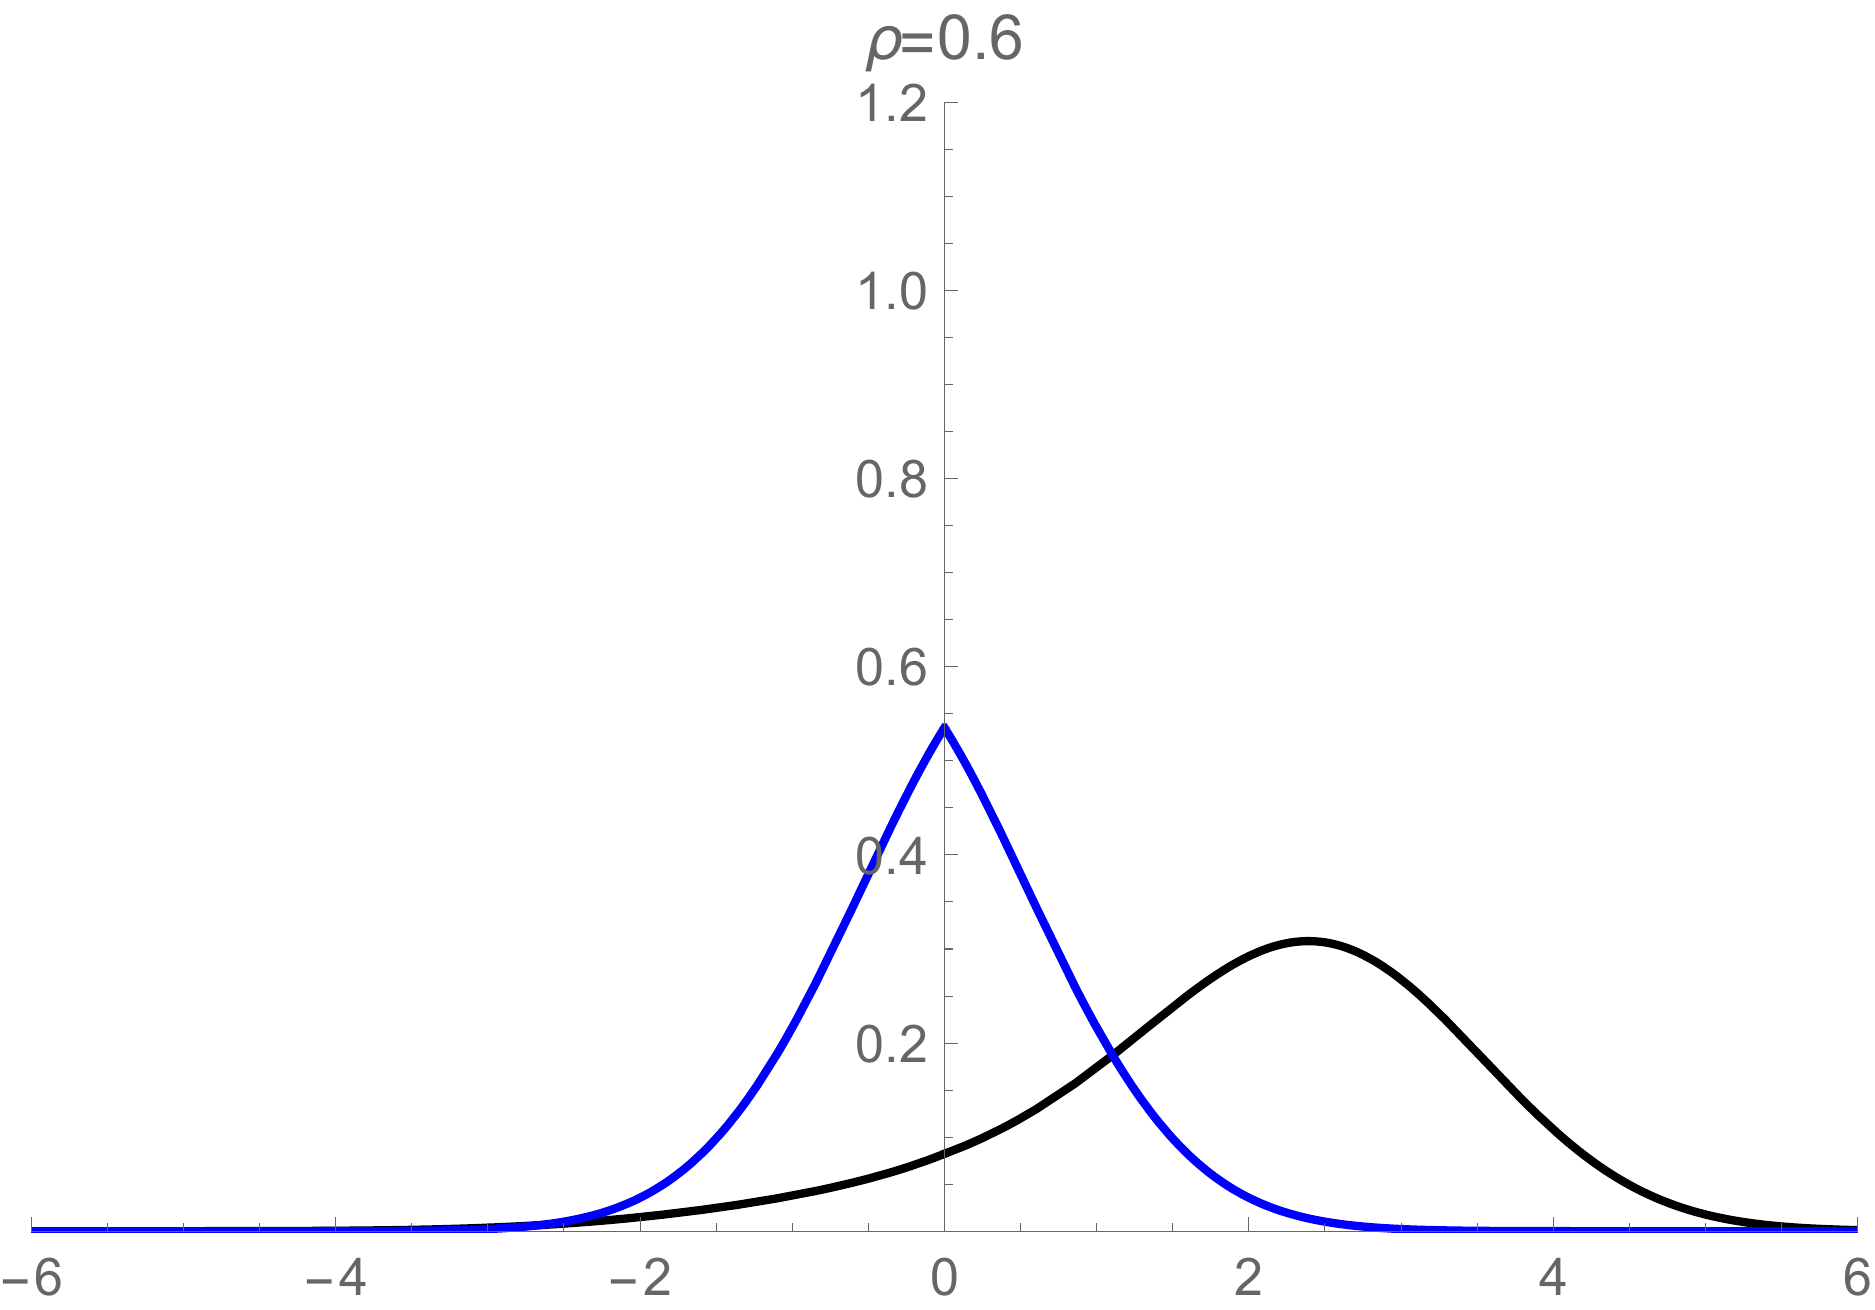}
         \caption{$\rho=0.6$}
     \end{subfigure}
     \hfill
     \begin{subfigure}[b]{0.3\textwidth}
         \centering
         \includegraphics[width=\textwidth]{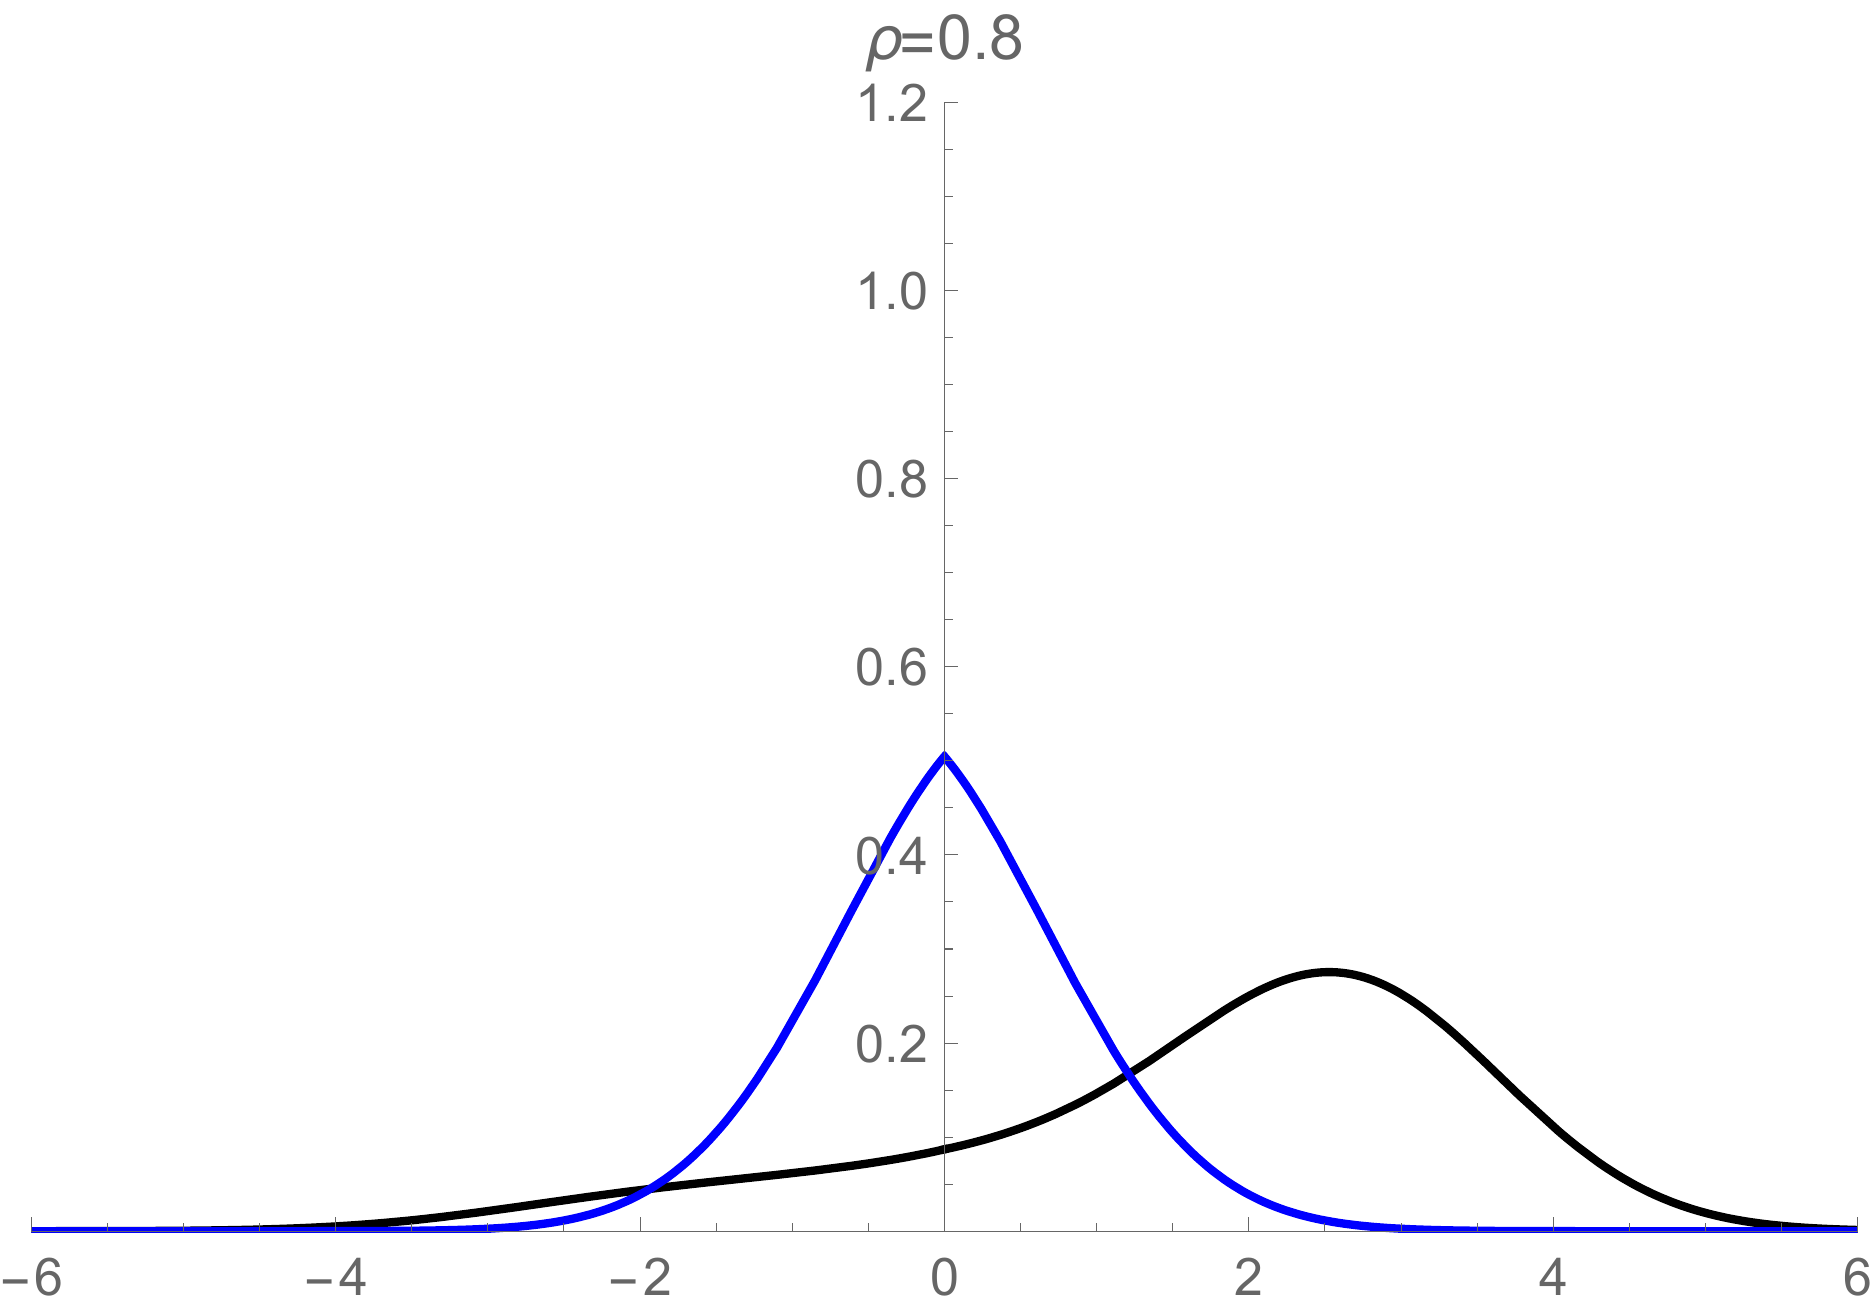}
         \caption{$\rho=0.8$}
     \end{subfigure}
     \hfill
     \begin{subfigure}[b]{0.3\textwidth}
         \centering
         \includegraphics[width=\textwidth]{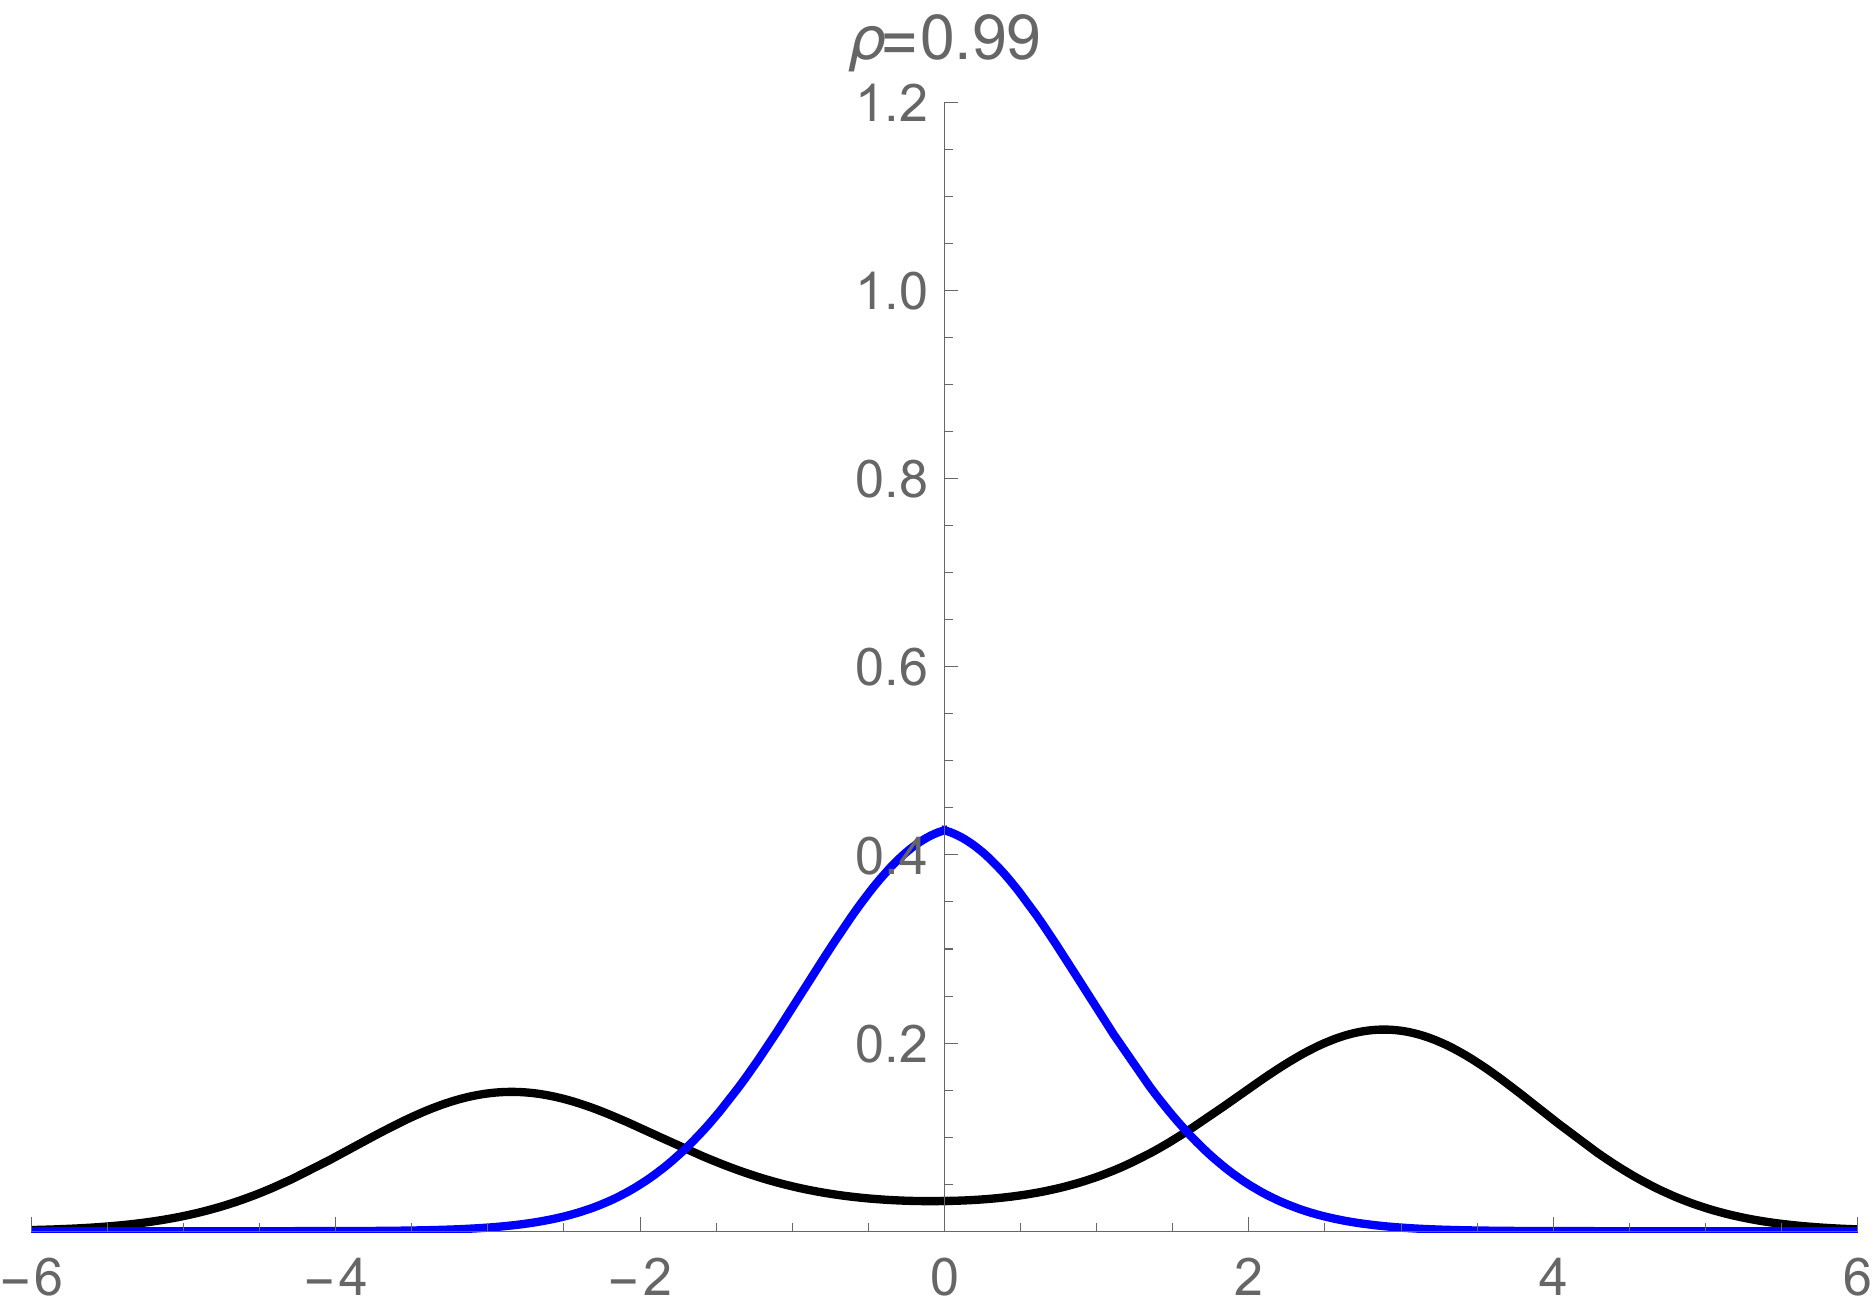}
         \caption{$\rho=0.99$}
     \end{subfigure}
        \caption{Comparison of $(1-\rho^2)^{-1/2}F_{h\sqrt{1-\rho^2},\rho}$ (black) and $F_{0,\rho}$ (blue) with $h=3$.}
        \label{fig:compare-rhos}
\end{figure}
